# Supplementary material for: Active-Dormant Attention Heads: Mechanistically Demystifying Extreme-Token Phenomena in LLMs
Source: arXiv:2410.13835 source file (2024-11-07)
Supplement: Supplementary file 6 [file proof.tex]

\section{Proofs}
\label{sec:proof}
Since we drop the trigger tokens in the loss function, we neglect $\cT$ throughout the proof for notational convenience, assuming that $\vocab$ consists of only non-trigger tokens.
We provide new notations which are frequently used in the proofs. Define the full bigram transition probability. 
\begin{equation}\label{appeqn:P-matrix}
\Transition = \left(\begin{matrix}
\transition_{11} & \ldots & \transition_{1\vocabsize}\\
\vdots & \ddots & \vdots \\
\transition_{\vocabsize 1} & \ldots & \transition_{\vocabsize\vocabsize}\\
\end{matrix}\right) = \left(\begin{matrix}
\bm{\transition}_1^\top\\
\vdots \\
\bm{\transition}_\vocabsize^\top\\
\end{matrix}\right).
\end{equation}
Given token $\tok$, define the predicted probability, which is the logit output passed through the softmax activation 
\begin{equation}\label{appeqn:pred-prob}
\bm{\ppred}_{\tok} = \softmax(\TF([\bos; v_{1:n-1}; v])_n).
\end{equation}
Similarly, define the full output probability matrix.
\begin{equation}\label{appeqn:Q-matrix}
\Ppred = \left(\begin{matrix}
\ppred_{11} & \ldots & \ppred_{1\vocabsize}\\
\vdots & \ddots & \vdots \\
\ppred_{\vocabsize 1} & \ldots & \ppred_{\vocabsize\vocabsize}\\
\end{matrix}\right) = \left(\begin{matrix}
\bm{\ppred}_1^\top\\
\vdots \\
\bm{\ppred}_\vocabsize^\top\\
\end{matrix}\right).
\end{equation}
Given any vector $\bm{u}=[u_1;\ldots;u_d]$, define the corresponding diagonal matrix as
\[
\diag(\bm{u}) = \left(\begin{matrix}
u_{1} & 0 & \ldots & 0\\
\vdots & \ddots &  & \vdots \\
\vdots & & \ddots & \vdots \\
0 & \ldots & 0 & u_d \\
\end{matrix}\right).
\]
Define 
\[
\gppred_\tok^{\Ppred} = \diag(\bm{\ppred}_\tok) - \bm{\ppred}_\tok \bm{\ppred}_\tok^\top \quad \gppred_\tok^{\Ppred} = \diag(\bm{\transition}_\tok) - \bm{\transition}_\tok \bm{\transition}_\tok^\top.
\]
Denote $\bm{z} = W \cdot \vecvalue - \bm{W} \circ \bm{\xi}$. We present a technical lemma.
\begin{lemma}\label{appthm:positive-definite}
The matrices $\gppred^\Transition_\tok$ and $\gppred^\Ppred_\tok$ are positive semi-definite for any $\tok$.
\end{lemma}
\begin{proof}
Since we have that $\sum_{\tokk=1}^\vocabsize \transition_{\tok\tokk} = 1$ and $\sum_{\tokk=1}^\vocabsize \ppred_{\tok\tokk} = 1$ for any $\tok$,
\begin{align*}
(\gppred^\Transition_\tok)_{\toki\toki}=\transition_\toki - \transition_{\toki}^2 & = \transition_\toki(\sum_{\tokk\neq\toki} \transition_\tokk) \geq \sum_{\tokk\neq\toki} |(\gppred^\Transition_\tok)_{\toki\tokk}| \\
(\gppred^\Ppred_\tok)_{\toki\toki}=\ppred_\toki - \ppred_{\toki}^2 & = \ppred_\toki(\sum_{\tokk\neq\toki} \ppred_\tokk) \geq \sum_{\tokk\neq\toki} |(\gppred^\Ppred_\tok)_{\toki\tokk}|.
\end{align*}
This shows that both $\gppred^\Transition_\tok$ and $\gppred^\Ppred_\tok$ are diagonally dominant matrices. By Corollary 6.2.27 in \citet{horn2012matrix}, they are positive semi-definite.
\end{proof}

\subsection{Proof of Theorem \ref{thm:construction}}\label{app:proof-construction}
We denote the hidden dimension as $d$ and the sequence length as $N$. We begin with the assumption regarding the transformer's positional embedding:
\begin{assumption}\label{ass:linear_indp}
For any token $\tok$ and position $\toki$, assume that the encoding combined with the positional embedding ensures that $\set{\embd(\tok_\toki)}$ is linearly independent.
\end{assumption}
Assumption \ref{ass:linear_indp} requires that $d\geq \vocabsize N$. Given the fact that there are  $O(\exp(d))$ approximately linearly independent vectors for large $d$ \citep{vershynin2018high}, it is possible to apply approximation theory to avoid Assumption \ref{ass:linear_indp}. However, since Assumption \ref{ass:linear_indp} pertains only to the construction of $\lambda$ for trigger tokens and is unrelated to Theorem \ref{thm:main}, we adopt it to simplify the proof of Theorem \ref{thm:construction}.

\begin{proof}
%  We concatenate the one-hot encoding $\bm{e}_\tok$ with $d-\vocabsize$ zeros, augmenting it to $\bm{e}_\tok\in\R^d$. Define the positional embeddings as $\Pos_\toki = [\bm{0}_{\vocabsize+1}; \br_\toki]$ for $\toki=0,\ldots,N$, with $\br_\toki \in \R^{d-\vocabsize-1}$ The input of the attention layer becomes 
% \[
% \embd(\tok_\toki) = \bm{e}_{\tok_\toki} + \Pos_\toki.
% \] 
% We define a matrix $\bA\in \R^{d\times d}$ such that $\bA\Pos_{\toki} = \Pos_{\toki-1}$ for $\toki\in[N]$ and $A \bm{e}_\tok=0$ for any $\tok\in\vocab$. Since $\{\bm{e}_\tok,\Pos_{\toki}\}_{\tok\in\vocab,\toki\leq N}$ is linear independent, the existence is guaranteed. Similarly, we define a matrix $\bB \in \R^{d\times d}$ such that $\bB \embd(\tok_{\toki}) = \bm{0}$ for any $\tok_\toki\in\cT$, $\bB \bm{e}_\tok = 0$ for any $\tok\in\vocab\setminus \cT$, and $(\lambda-1) \Pos_{\tokj}^\top \bB \Pos_{\toki} + \sink \Pos_{\tokj}^\top \bB \bm{e}_{\bos}=0$. \tianyu{check}
% Define the value, key, and query matrices as 
% \[
% V = \sum_{\tok\in\vocab\setminus\cT}
% \]

% Then, we have that 
% We augment the one-hot encoding $\bm{e}_\tok$ to $\R^d$, concatenating it with $d-\vocabsize$ zeros. 
Consider vectors $\bu_{i}\in\R^d$, $i\in[N]$ such that $\bu_i^\top\bu_j=0$, $i\neq j$, and $\bu_i^\top\embd(\tok_j)$ for any $\tok\in\vocab$ and $i$, $j\in[N]$.
Adopting Assumption \ref{ass:linear_indp}, there exists a matrix $\query$ such that
\begin{equation}\label{appeqn:mlp-construct}
\begin{aligned}
&~\query(\embd(\tok_i)) = \lambda\bu_{i-1}~~~\text{for }\tok_i\in\cT,~~i>1,\\
&~\query(\embd(\tok_i)) = \sink_{\tok_i} \bu_{0}~~~\text{for }\tok_i\in\vocab\setminus\cT,~~i>0.\\
\end{aligned}
\end{equation}
Define the corresponding key matrix.
\begin{equation}
\begin{aligned}
&~\key(\embd(\tok_i)) =  \bu_{i}~~~\text{for }\tok_i\in\vocab,~~i> 0,\\
&~\key(\embd(\bos)) = \bu_{0}.
\end{aligned}
\end{equation}
There exists a value matrix $\val{}$ such that
\begin{equation}
\begin{aligned}
&~\val(\embd(\tok_i)) = 0~~~\text{for }\tok_i\in\cT,~~i> 1,\\
&~\val(\embd(\tok_i)) = \xi_{\tok_i}\bu_{i}~~~\text{for }\tok_i\in\vocab\setminus\cT,~~i> 0,\\
&~\val(\embd(\bos)) = \vecvalue.\\
\end{aligned}
\end{equation}
Further define the matrix $\bM$ that satisfies
\begin{equation}
\begin{aligned}
&~ \bM (\embd(\tok_i)) = \log \bp_{\tok_i} \cdot 1\{ \tok_i \not\in \cT  \}  ~~~ \text{for } \tok_i \in \vocab,~~i\in[N],\\
&~ \bM  (\bu_i) = \bm{e}_i ~~~ \text{for }i\in[N].
\end{aligned}
\end{equation}
Setting $\mlp(\cdot)=\text{ReLU}(\bM (\cdot))$, we can then verify that the residual connection gives that $\TF([\bos; v_{1:n-1}; v_n])=\mlp(\embd(\tok_n)+\attn(\embd(\tok_n)))$, which is equivalent to the simplified model. 

When $\min_{v \in \vocab} \sink_v \to\infty$, $\min_{v \in \vocab} \xi_v \to\infty$, $\lambda\to \infty$, and $\vecvalue=0$, if $v_n\in\cT$, $\softmax[\TF([\bos; v_{1:n-1}; v_n])] = \delta_{\tok_{n-1}}$. If $\tok_{n}\in\vocab\setminus\cT$, $\softmax[\TF([\bos; v_{1:n-1}; v_n])] = \bm{\transition}_{\tok_n}$. All next-token probabilities match those in the data-generating procedure, aligning with the oracle algorithm.
\end{proof}

\subsection{The stable phase in  Theorem \ref{thm:main}}\label{app:proof-main}

Lemma \ref{appthm:g-ppred} computes the gradient of $\Ppred$.
\begin{lemma}\label{appthm:g-ppred} 
We have
\begin{align*}
\frac{\partial \ppred_{\toki\tokk}}{\partial \sink_\tok} = &~ \frac{\bm{1}\{\toki=\tok\} \ppred_{\toki\tokk}e^{\sink_\toki}}{(e^{\sink_\toki}+W)^2} \Big[W\ivalue_\tokk-W_\tokk \xi_\tokk - \sum_{\tokj=1}^\vocabsize \ppred_{\toki\tokj} (W\ivalue_\tokj - W_\tokj\xi_\tokj)\Big],\\
\frac{\partial \ppred_{\toki\tokk}}{\partial \ivalue_\tok} = &~ \frac{e^{\sink_\toki}}{e^{\sink_\toki}+W}[\ppred_{\toki\tokk}\bm{1}\{\tokk=\tok\} - \ppred_{\toki\tokk}\ppred_{\toki\tok}].\\
\end{align*}
Furthermore,
\[
\sum_{\tokk=1}^\vocabsize \frac{\partial \ppred_{\toki\tokk}}{\partial \sink_\tok} = 0, \quad \sum_{\tok=1}^\vocabsize \frac{\partial \ppred_{\toki\tokk}}{\partial \ivalue_\tok} = 0.
\]
\end{lemma}
\begin{proof}
We repeatedly use the following two facts:
\begin{align*}
\frac{\partial\Big\{\exp\Big[\frac{W_\tokk\xi_\tokk+e^{\sink_\toki}\ivalue_\tokk}{e^{\sink_\toki}+W}\Big]\Big\}}{\partial \sink_\tok} = &~ \frac{\bm{1}\{\toki=\tok\}e^{\sink_\toki}(W\ivalue_\tokk-W_\tokk\xi_\tokk)}{(e^{\sink_\toki}+W)^2} \exp\Big[\frac{W_\tokk\xi_\tokk+e^{\sink_\toki}\ivalue_\tokk}{e^{\sink_\toki}+W}\Big],
\nonumber\\
\frac{\partial\Big\{\exp\Big[\frac{W_\tokk\xi_\tokk+e^{\sink_\toki}\ivalue_\tokk}{e^{\sink_\toki}+W}\Big]\Big\}}{\partial \ivalue_\tok} = &~ \frac{\bm{1}\{\tokk=\tok\}e^{\sink_\toki}}{e^{\sink_\toki}+W} \exp\Big[\frac{W_\tokk\xi_\tokk+e^{\sink_\toki}\ivalue_\tokk}{e^{\sink_\toki}+W}\Big].
\nonumber
\end{align*}

When $\toki\neq \tok$, $\ppred_{\toki\tokk}$ does not include $\sink_\tok$, making the gradients as zero. When $\toki=\tok$, we have
\begin{align*}
\frac{\partial \ppred_{\tok\tokk}}{\partial \sink_\tok} = &~ \ppred_{\tok\tokk} e^{\sink_\tok} \Big[\frac{W\ivalue_\tokk-W_\tokk\xi_\tokk}{(e^{\sink_\tok}+W)^2}\Big] - \frac{\ppred_{\tok\tokk}\sum_{\toki=1}^\vocabsize \transition_{\tok\toki} e^{\sink_\tok} \Big[\frac{W\ivalue_\toki-W_\toki\xi_\toki}{(e^{\sink_\tok}+W)^2}\Big]\exp\Big[\frac{W_\toki\xi_\toki+e^{\sink_\tok}\ivalue_\toki}{e^{\sink_\tok}+W}\Big]}{\sum_{\toki=1}^\vocabsize \transition_{\tok\toki}\exp\Big[\frac{W_\toki\xi_\toki+e^{\sink_\tok}\ivalue_\toki}{e^{\sink_\tok}+W}\Big]}\\
= &~ \frac{e^{\sink_\tok}}{(e^{\sink_\tok}+W)^2} \Big\{ \ppred_{\tok\tokk} [W\ivalue_\tokk-W_\tokk \xi_\tokk] - \ppred_{\tok\tokk}\sum_{\tokj=1}^\vocabsize \ppred_{\tok\tokj} (W\ivalue_\tokj - W_\tokj\xi_\tokj)\Big\},
\end{align*}
and
\begin{align*}
\frac{\partial \ppred_{\toki\tokk}}{\partial \ivalue_\tok} = &~ \Big[\frac{e^{\sink_\toki}}{e^{\sink_\toki}+W}\Big]\ppred_{\toki\tokk} \bm{1}\{\tokk=\tok\} - \frac{\Big[\frac{e^{\sink_\toki}}{e^{\sink_\toki}+W}\Big]\transition_{\toki\tok}\exp\Big[\frac{W_\tok\xi_\tok+e^{\sink_\toki}\ivalue_\tok}{e^{\sink_\toki}+W}\Big]\transition_{\toki\tokk}\exp\Big[\frac{W_\tokk\xi_\tokk+e^{\sink_\toki}\ivalue_\tokk}{e^{\sink_\toki}+W}\Big]}{\Big(\sum_{j=1}^\vocabsize \transition_{\toki\tokj}\exp\Big[\frac{W_\tokj\xi_\tokj+e^{\sink_\toki}\ivalue_\tokj}{e^{\sink_\toki}+W}\Big]\Big)^2}\\
= &~ \Big[\frac{e^{\sink_\toki}}{e^{\sink_\toki}+W}\Big] [ \ppred_{\toki\tokk} \bm{1}\{\tokk=\tok\} - \ppred_{\toki\tokk} \ppred_{\toki\tok} ].
\end{align*}
We can verify that 
\begin{align*}
\sum_{\tokk=1}^\vocabsize \frac{\partial \ppred_{\toki\tokk}}{\partial \sink_\tok} = &~  \frac{e^{\sink_\tok}}{(e^{\sink_\tok}+W)^2} \sum_{\tokk=1}^\vocabsize \Big\{ \ppred_{\tok\tokk} [W\ivalue_\tokk-W_\tokk \xi_\tokk] - \ppred_{\tok\tokk}\sum_{\tokj=1}^\vocabsize \ppred_{\tok\tokj}^\top (W\sink_\tokj - W_\tokj\xi_\tokj)\Big\}\\
= &~ \frac{e^{\sink_\tok}}{(e^{\sink_\tok}+W)^2}  \Big\{\sum_{\tokk=1}^\vocabsize \ppred_{\tok\tokk} [W\ivalue_\tokk-W_\tokk \xi_\tokk] - \sum_{\tokj=1}^\vocabsize \ppred_{\tok\tokj}^\top (W\sink_\tokj - W_\tokj\xi_\tokj)\Big\}\\
= &~ 0,
\end{align*}
and
\begin{align*}
\sum_{\tok=1}^\vocabsize \frac{\partial \ppred_{\toki\tokk}}{\partial \ivalue_\tok} = &~   \Big[\frac{e^{\sink_\toki}}{e^{\sink_\toki}+W}\Big] \sum_{\tok=1}^\vocabsize [\ppred_{\toki\tokk} \bm{1}\{\tokk=\tok\} - \ppred_{\toki\tokk} \ppred_{\toki\tok} ]\\
= &~ \Big[\frac{e^{\sink_\toki}}{e^{\sink_\toki}+W}\Big] [\ppred_{\toki\tokk} - \ppred_{\toki\tokk} ]\\
= &~ 0.
\end{align*}
This finishes the proof of Lemma \ref{appthm:g-ppred}.
\end{proof}

Proposition \ref{appthm:gradients} computes the gradient of $\loss$ with respect to $\vecsink$ and $\vecvalue$, giving the gradient flow.
\begin{proposition}\label{appthm:gradients}
The gradient flow of optimizing $\loss(\vecsink, \vecvalue)$ is given by
\begin{align*}
\dot{\sink}_\tok(t) & = \frac{\stable_\tok e^{\sink_\tok}}{(e^{\sink_\tok}+W)^2} 
\sum_{\toki=1}^\vocabsize({\transition}_{\tok\toki}-{\ppred}_{\tok\toki})(W\ivalue_\toki-W_\toki\xi_\toki),\\
\dot{\ivalue}_\tok(t) & = \sum_{\tokk=1}^\vocabsize \Big\{\frac{\stable_\tokk e^{\sink_\tokk} [\transition_{\tokk\tok} - \ppred_{\tokk\tok}]}{e^{\sink_\tokk}+W}\Big\}.
\end{align*}
\end{proposition}
\begin{proof}
The gradient flow gives that
\[
\dot{\sink}_\tok(t) = - \frac{\partial \loss(\vecsink,\vecvalue)}{\partial \sink_\tok}, \quad \text{and}\quad \dot{\ivalue}_\tok(t)=-\frac{\partial\loss(\vecsink, \vecvalue)}{\partial \ivalue_\tok}.
\]
Taking the derivative of $\loss(\vecsink,\vecvalue)$ gives that
\begin{align*}
\frac{\partial \loss(\vecsink,\vecvalue)}{\partial \sink_\tok}
= ~& \stable_\tok \sum_{\tokk=1}^\vocabsize \transition_{\tok\tokk} \cdot \frac{-1}{\ppred_{\tok\toki}}\cdot \frac{\partial \ppred_{\tok\toki}}{\partial \sink_\tok}\\
= ~& \frac{\stable_\tok e^{\sink_\tok}}{(e^{\sink_\tok}+W)^2} \Big\{  \sum_{\toki=1}^\vocabsize \ppred_{\tok\toki} [W\ivalue_\toki - W_\toki \xi_\toki] - \sum_{\tokk=1}^\vocabsize \transition_{\tok\tokk} [W\ivalue_\tokk-W_\tokk\xi_\tokk]\Big\}\\
= ~& \frac{\stable_\tok e^{\sink_\tok}}{(e^{\sink_\tok}+W)^2} \sum_{\tokk=1}^\vocabsize \Big\{  [\ppred_{\tok\tokk}-\transition_{\tok\tokk}] [W\ivalue_\tokk-W_\tokk\xi_\tokk]\Big\}.
\end{align*}
Similarly, we have that
\begin{align*}
\frac{\partial \loss(\vecsink,\vecvalue)}{\partial \ivalue_\tok} 
= ~& \sum_{j=1}^\vocabsize \stable_\tokj \sum_{\tokk=1}^\vocabsize \transition_{\tokj\tokk} \Big\{ \frac{e^{\sink_\tokj} \ppred_{\tokj\tok}}{e^{\sink_\tokj}+W} - \frac{e^{\sink_\tokj} \bm{1}\{\tokk=\tok\}}{e^{\sink_\tokj}+W} \Big\}\\
= ~& \sum_{j=1}^\vocabsize \Big\{\frac{\stable_{\tokj}e^{\sink_\tokj}[\ppred_{\tokj\tok}-\transition_{\tokj\tok}]}{e^{\sink_\tokj}+W}\Big\}.
\end{align*}
This proves Proposition \ref{appthm:gradients}.
\end{proof}
% \begin{theorem}[Restatement of Theorem \ref{thm:main}]\label{appthm:main}
% Consider the gradient flow of optimizing $\loss(\vecsink, \vecvalue)$. We have that 
% \begin{enumerate}
%     \item (identical attention logits) The gradient flow has equilibria 
%     \[\vecsink = \sink \bm{1}, \quad \vecvalue = c \cdot \bm{1} - e^{-\sink} \cdot \bm{W}\circ \bm{\xi}.\]
%     \item (\textit{attention sink}) Fixing $\vecvalue= c \cdot \bm{1}$, with any initial value $\vecsink(0)$, there exists $\bm{r}(t)$ with bounded norm such that
%     \[\vecsink(t) = \frac{1}{2} \log t \cdot \bm{1} + \bm{r}(t).\]
%     \item (\textit{small value states}) Fixing $\vecsink = \sink \cdot \bm{1}$, with any initial value $\vecvalue(0)$, we have for any $\toki$,
%     \[\abs{\ivalue_\toki(t) - \bar\ivalue(0) - e^{-\sink} W_\toki \xi_\toki} \leq \delta e^{-\mu t},\]
%     where $\bar{\ivalue}(0) = V^\inv[\sum_{\tok} \ivalue_\tok(0)]$, $\delta>0$, and $\mu>0$.
% \end{enumerate}
% \end{theorem}
\begin{theorem}[Restatement the stable phase part in Theorem \ref{thm:main}]\label{appthm:main-1}
Consider the gradient flow of optimizing $\loss(\vecsink, \vecvalue)$. The gradient flow has sink stationary points 
\[\vecsink^\star = \sink \bm{1}, \quad \vecvalue^\star = c \cdot \bm{1} - e^{-\sink} \cdot \bm{W}\circ \bm{\xi}.\]
\end{theorem}
\begin{proof}
When $\vecsink=\vecsink^\star$ and $\vecvalue=\vecvalue^\star$, 
\begin{align*}
\ppred_{\tok\toki} = &~ \frac{\transition_{\tok\toki} \exp\Big[\frac{W_\toki\xi_\toki+e^{\sink}\ivalue_\toki}{e^{\sink}+W}\Big]}{\sum_{\tokk=1}^\vocabsize \transition_{\tok\tokk}\exp\Big[\frac{W_\tokk\xi_\tokk+e^{\sink}\ivalue_\tokk}{e^{\sink}+W}\Big]} \\
 = &~ \frac{\transition_{\tok\toki} \exp\Big[\frac{c}{e^{\sink}+W}\Big]}{\sum_{\tokk=1}^\vocabsize \transition_{\tok\tokk}\exp\Big[\frac{c}{e^{\sink}+W}\Big]} \\
 = &~ \transition_{\tok\toki}.
\end{align*}
Take $\ppred_{\tok\toki}$'s into $\partial \loss(\vecsink,\vecvalue)/\partial \vecsink$ and $\partial \loss(\vecsink,\vecvalue)/\partial \vecvalue$.
\begin{align*}
\frac{\partial \loss(\vecsink,\vecvalue)}{\partial \sink_\tok}\Big |_{\vecsink^\star,\vecvalue^\star} & = \frac{\stable_\tok e^{\sink_\tok}}{(e^{\sink_\tok}+W)^2} 
\sum_{\tokk=1}^\vocabsize \Big\{(\ppred_{\tok\tokk}-\transition_{\tok\tokk}) [W \ivalue_\tokk - W_\tokk \xi_\tokk]
\Big\} = 0,\\
\frac{\partial \loss(\vecsink,\vecvalue)}{\partial \ivalue_\tok}\Big |_{\vecsink^\star,\vecvalue^\star} & = \sum_{\tokk=1}^\vocabsize \Big\{\frac{\stable_\tokk e^{\sink_\tokk} [\ppred_{\tokk\tok}-\transition_{\tokk\tok} ]}{e^{\sink_\tokk}+W}\Big\} = 0.
\end{align*}
This shows that the given points are stationary points. We further compute the second-order derivative using Lemma \ref{appthm:g-ppred}. Define $\bz=[z_1;\ldots;z_\vocabsize]$ so that $z_\tokk = W \ivalue_\tokk - W_\tokk \xi_\tokk$.
\begin{align*}
\frac{\partial^2 \loss(\vecsink, \vecvalue)}{\partial \sink_\toki \partial \sink_\tok} \Big |_{\vecsink^\star,\vecvalue^\star} =  ~& \bm{1}\{\tok=\toki\}\cdot \frac{\stable_\tok e^{\sink}}{(e^{\sink}+W)^2} 
\sum_{\tokk=1}^\vocabsize \Big\{\frac{\partial \ppred_{\toki\tokk}}{\partial \sink_\tok} z_\tokk
\Big\}\\
=  ~& \bm{1}\{\tok=\toki\}\cdot \frac{\stable_\tok e^{2\sink}}{(e^{\sink}+W)^4} 
\Big\{ \sum_{\tokk=1}^\vocabsize \ppred_{\toki\tokk} z_\tokk^2 - \Big[\sum_{\tokk=1}^\vocabsize \ppred_{\toki\tokk}z_\tokk \Big]^2
\Big\},\\
=  ~& \bm{1}\{\tok=\toki\}\cdot \frac{\stable_\tok e^{2\sink}}{(e^{\sink}+W)^4} 
\Big\{ \sum_{\tokk=1}^\vocabsize \transition_{\toki\tokk} z_\tokk^2 - \Big[\sum_{\tokk=1}^\vocabsize \transition_{\toki\tokk}z_\tokk \Big]^2
\Big\}.
\end{align*}
where in the last line, we take $\Ppred=\Transition$. Similarly, we compute the gradients with respect to $\sink_\toki$ and $\ivalue_\tok$.
\begin{align*}
\frac{\partial^2 \loss(\vecsink, \vecvalue)}{\partial \sink_\toki \partial \ivalue_\tok} \Big |_{\vecsink^\star,\vecvalue^\star} =  ~& \frac{\stable_\toki e^{\sink}}{(e^{\sink}+W)^2} 
\sum_{\tokk=1}^\vocabsize \Big\{\frac{\partial \ppred_{\toki\tokk}}{\partial \ivalue_\tok} z_\tokk
\Big\}\\
=  ~& \frac{\stable_\toki e^{2\sink}}{(e^{\sink}+W)^3} 
\Big\{ \transition_{\toki\tok} z_\tokk - \transition_{\toki\tok} \sum_{\tokk=1}^\vocabsize  \transition_{\toki\tokk}z_\tokk
\Big\}.
\end{align*}
With the same manner, we compute the gradients with respect to $\ivalue_\toki$ and $\ivalue_\tok$.
\begin{align*}
\frac{\partial^2 \loss(\vecsink, \vecvalue)}{\partial \ivalue_\toki \partial \ivalue_\tok} \Big |_{\vecsink^\star,\vecvalue^\star} =  ~& \sum_{\tokk=1}^\vocabsize \Big\{\frac{\partial \ppred_{\tokk\toki}}{\partial \ivalue_\tok}\frac{\stable_\tokk e^{\sink}}{e^{\sink}+W}\Big\}\\
= ~& \frac{e^{2\sink}}{(e^\sink+W)^2}\sum_{\tokk=1}^\vocabsize \{ \stable_\tokk [\bm{1}\{\tok=\toki\} \transition_{\tokk\tok} - \transition_{\tokk\toki}\transition_{\tokk\tok}] \}.
\end{align*}
Combining the above computations gives that
\begin{align*}
\text{Hessian}(\loss(\vecsink^\star, \vecvalue^\star)) = \left(\begin{matrix}
\nabla^2_{\vecsink} \loss(\vecsink,\vecvalue) & \nabla_{\vecsink} \nabla_{\vecvalue}  \loss(\vecsink,\vecvalue)\\
\nabla_{\vecvalue} \nabla_{\vecsink} \loss(\vecsink,\vecvalue) & \nabla^2_{\vecsink} \loss(\vecsink,\vecvalue)\\
\end{matrix}\right),
\end{align*}
with
\begin{align*}
\nabla^2_{\vecsink} \loss(\vecsink,\vecvalue) = &~ \frac{e^{2\sink}}{(e^\sink+W)^4}\diag\Big\{ \stable \circ [\bz^\top \gppred^\Transition_1\bz;\ldots;\gppred^\Transition_\vocabsize \bz] \Big\},\\
\nabla_{\vecsink} \nabla_{\vecvalue} \loss(\vecsink,\vecvalue) = &~ \frac{e^{2\sink}}{(e^\sink+W)^3}\diag\Big\{ \stable \Big\} [ \bz^\top\gppred^\Transition_1;\ldots; \bz^\top\gppred^\Transition_\vocabsize] ,\\
\nabla^2_{\vecvalue} \loss(\vecsink,\vecvalue) = &~ \frac{ e^{2\sink}}{(e^{\sink}+W)^2} \sum_{\tokk=1}^\vocabsize  \stable_\tokk \gppred^\Transition_\tokk.\\
\end{align*}
At last, we diagonalize the Hessian matrix and get that
\[
\text{Diag-Hessian}(\loss(\vecsink^\star, \vecvalue^\star)) = \left(\begin{matrix}
\nabla^2_{\vecsink} \loss(\vecsink,\vecvalue) & 0\\
0 & \frac{ e^{2\sink}}{(e^{\sink}+W)^2} \bH\\
\end{matrix}\right),
\]
where the $\bH$ is given by
\begin{align*}
\bH = \sum_{\tokk=1}^\vocabsize  \stable_\tokk \Big(\gppred^\Transition_\tokk - (\bm{z}^\top \gppred_\tokk^\Transition \bm{z})^{-1}\gppred^\Transition_\tokk\bm{z}\bm{z}^\top\gppred^\Transition_\tokk\Big).
\end{align*}
To prove that $\bH$ is positive semi-definite, consider any vector $\bm{\eta}$ with $\|\bm{\eta}\|_2=1$.
\begin{align*}
\bm{\eta}^\top \bH \bm{\eta} = &~ \sum_{\tokk=1}^\vocabsize  \stable_\tokk \Big(\bm{\eta}^\top\gppred^\Transition_\tokk\bm{\eta} - \frac{\bm{\eta}^\top\gppred^\Transition_\tokk\bm{z}\bm{z}^\top\gppred^\Transition_\tokk\bm{\eta}}{\bm{z}^\top \gppred_\tokk^\Transition \bm{z}}\Big).
\end{align*}
Since $\gppred^\Transition_\tokk$'s are positive semi-definite, the Cauchy inequality gives that
\[
\bm{z}^\top\gppred^\Transition_\tokk\bm{\eta} \leq \sqrt{\bm{z}^\top \gppred_\tokk^\Transition \bm{z} \bm{\eta}^\top \gppred_\tokk^\Transition \bm{\eta}}.
\]
As a result, we have that
\begin{align*}
\bm{\eta}^\top \bH \bm{\eta} \geq &~ \sum_{\tokk=1}^\vocabsize  \stable_\tokk \Big(\bm{\eta}^\top\gppred^\Transition_\tokk\bm{\eta} - \frac{\bm{z}^\top \gppred_\tokk^\Transition \bm{z} \bm{\eta}^\top \gppred_\tokk^\Transition \bm{\eta}}{\bm{z}^\top \gppred_\tokk^\Transition \bm{z}}\Big) = 0.
\end{align*}
This shows that $\bH$ is positive semi-definte. Therefore, $\text{Hessian}(\loss(\vecsink^\star, \vecvalue^\star))$ is positive semi-definte. This proves Theorem \ref{appthm:main-1}.
\end{proof}
We prove Theorem \ref{appthm:main-1} through direct computation. Due to the non-linearity, it's unclear whether other stationary points exist. However, we observe that all of our simulations converge to the given stationary points. 
\subsection{Attention sinks in Theorem \ref{thm:main}}
\begin{theorem}[Restatement of the attention sink part in Theorem \ref{thm:main}]\label{appthm:main-2}
Fixing $\vecvalue= c \cdot \bm{1}$, with any initial value, there exists $\bm{r}(t)$ with bounded norm such that
\[\vecsink(t) = \frac{1}{2} \log t \cdot \bm{1} + \bm{r}(t).\]
\end{theorem}
\begin{proof}
We separately analyze each entry of $\vecsink$. Focusing on $\sink_\tok$, to simplify the notation, we introduce a random variable $\varphi$ such that $\P(\varphi=W_\tokk\xi_\tokk)=\transition_{\tok\tokk}$.
Define 
\[
u = e^{\sink_\tok}.
\]
Therefore, using Lemma \ref{appthm:gradients}, we get that
\begin{align*}
\frac{\mathrm{d} u}{\mathrm{d} t} = \frac{\stable_\tok e^{2\sink_\tok}}{(e^{\sink_\tok}+W)^2} 
\sum_{\toki=1}^\vocabsize({\ppred}_{\tok\toki}-{\transition}_{\tok\toki})(W\ivalue_\toki-W_\toki\xi_\toki).
\end{align*}
We take in $\ivalue = c$ and expand the expression of $\mathrm{d}u/\mathrm{d}t$. This gives us
\begin{align*}
\frac{\mathrm{d} u}{\mathrm{d} t} = &~ \frac{\stable_\tok u^2}{(u+W)^2} \frac{\sum_{\tokk=1}^\vocabsize \transition_{\tok\tokk} e^{W_\tokk\xi_\tokk/(u+W)}W_\tokk\xi_\tokk - \sum_{\tokk=1}^\vocabsize \transition_{\tok\tokk} e^{W_\tokk\xi_\tokk/(u+W)}\sum_{\tokk=1}^\vocabsize W_\tokk\xi_\tokk}{\sum_{\tokk=1}^\vocabsize \transition_{\tok\tokk} e^{W_\tokk\xi_\tokk/(u+W)}}\\
= &~ \frac{\stable_\tok u^2}{(u+W)^2} \frac{\Cov(e^{\frac{\varphi}{u+W}},\varphi)}{\E e^{\frac{\varphi}{u+W}}}.
\end{align*}
Since both $e^{x/(u+W)}$ and $x$ are monotonically increasing with respect to $x$, $u$ is monotonically increasing. This means that
\[
\frac{u(t)^2}{[u(t)+W]^2} \geq \frac{u(0)^2}{[u(0)+W]^2},\quad \E e^{\frac{\varphi}{u(t)+W}} \leq \E e^{\frac{\varphi}{u(0)+W}}.
\]
Meanwhile, if we consider the first and second order approximation of $e^{\varphi/(u+W)}$, 
\[
e^{\frac{\varphi}{u+W}} = 1 + \frac{\theta_1(\varphi) \varphi}{u+W},\quad e^{\frac{\varphi}{u+W}} = 1 + \frac{\varphi}{u+W} + \theta_2(\varphi) \Big[\frac{\varphi}{u+W}\Big]^2.
\]
Both $\theta_1(\varphi)$ and $\theta_2(\varphi)\varphi^2$ are  monotonically increasing functions of $\varphi$. We also have the bound
\[
\theta(\varphi) \leq \frac{e^{\frac{\max \varphi}{u(0)+W}}-1}{\frac{\max \varphi}{u(0)+W}-1} = C_\theta.
\]
Therefore, we get two more inequalities
\[
\Cov(\theta_1(\varphi)\varphi,\varphi)\leq C_\theta \Var(\varphi),\quad \Cov(\theta_2(\varphi)\varphi^2,\varphi)\geq 0.
\]
With all the preparatory works down, we give upper and lower bounds for $\mathrm{d}u/\mathrm{d}t$.
We first upper-bound $\mathrm{d}u/\mathrm{d}t$. 
\begin{align*}
\frac{\mathrm{d}u}{\mathrm{d}t} \leq &~ \stable_\tok \Cov(e^{\frac{\varphi}{u+W}}, \varphi)\\
= &~ \stable_\tok\Cov(1 + \frac{\theta_1(\varphi)\varphi}{u+W}, \varphi)\\
\leq &~ \frac{\stable_\tok C_\theta \Var(\varphi)}{u}.
\end{align*}
By solving the corresponding ODE, we get that
\begin{align*}
\frac{1}{2} u^2 \leq \sqrt{C_\theta \Var(\varphi) t} + C.
\end{align*}
To give a lower bound, we have that
\begin{align*}
\frac{\mathrm{d}u}{\mathrm{d}t} \geq &~ \frac{u(0)^2}{[u(0)+W]^2}\frac{\stable_\tok \Cov(e^{\frac{\varphi}{u+W}},\varphi)}{\E e^{\frac{\varphi}{u(0)+W}}} \\
\geq &~ \frac{u(0)^2}{[u(0)+W]^2}\frac{\stable_\tok}{\E e^{\frac{\varphi}{u(0)+W}}} \Cov(1+\frac{\varphi}{u+W}+\theta_2(\varphi) \Big[\frac{\varphi}{u+W}\Big]^2,\varphi)\\
\geq &~ \frac{u(0)^2}{[u(0)+W]^2}\frac{\stable_\tok}{\E e^{\frac{\varphi}{u(0)+W}}} \frac{\Var(\varphi)}{u+W}\\
\geq &~ \frac{u(0)^2}{[u(0)+W]^2}\frac{\stable_\tok}{\E e^{\frac{\varphi}{u(0)+W}}} \cdot \frac{u(0)}{u(0)+W} \cdot \frac{\Var(\varphi)}{u}\\
= &~ \Tilde{C}_\theta \frac{1}{u}.
\end{align*}
Therefore, $u \geq \sqrt{\Tilde{C}_\theta t + \Tilde{C}}$. In conclusion, 
\[
y_{\tok} = \log u = \frac{1}{2}\log t + r_{\tok},
\]
with $r_{\tok}$ bounded.
\end{proof}
\subsection{Value state drains in Theorem \ref{thm:main}}
\begin{theorem}[Restatement of Theorem \ref{thm:main}]\label{appthm:main-3}
Fixing $\vecsink=y\bm{1}$, $\vecvalue=c\bm{1}-e^{-\sink} \bm{W}\circ \bm{\xi}$ with $c\in\R$. Define $\bar{\ivalue}(t)=\vocabsize^{-1}\sum_{\toki=1}^\vocabsize \ivalue_\toki(t)$. Then the gradient flow of $\vecvalue(t)$ converges:
\[
\vecvalue(t) \to \vecvalue^\star=\bar{\ivalue}(0)\bm{1}-e^{-\sink} \bm{W}\circ \bm{\xi}.
\]
\end{theorem}
\begin{proof}
Theorem \ref{appthm:main-1} has already verified that $\vecvalue=c\bm{1}-e^{-\sink} \bm{W}\circ \bm{\xi}$ are stationary points of $\loss$.
In the proof of Theorem \ref{appthm:main-1}, we have derived $\nabla^2_{\vecvalue} \loss(\vecsink,\vecvalue)$.
\begin{align*}
\nabla^2_{\vecvalue} \loss(\vecsink,\vecvalue) = \sum_{\tokk=1}^\vocabsize \stable_\tokk \gppred^\Ppred_\tokk.
\end{align*}
Lemma \ref{appthm:positive-definite} indicates that it is positive semi-definite. Therefore, all stationary points attain the minimum of $\loss(\vecsink,\vecvalue)$. Suppose $\vecvalue^\star$ is a stationary point, we therefore get that $\ppred_{\tok\tokk}=\transition_{\tok\tokk}$ for any $\tok,$ $\tokk$. This implies that $e^y \ivalue^\star_\tokk + W_\tokk \xi_\tokk$ are constants across $\tokk$. We can solve $\ivalue^\star$ and get that
$\vecvalue^\star=c\bm{1}-e^{-\sink} \bm{W}\circ \bm{\xi}$. The convexity of the $\loss(\vecsink,\vecvalue)$ guarantees that $\vecvalue$ always converges to a stationary point $\vecvalue^\star$.

To find the value of $c$ in $\vecvalue^\star$, note that  $\sum_{\tok=1}^\vocabsize \dot{\ivalue}_\tok(t)=0$. We get that $\bar{\ivalue}^\star=\bar{\ivalue}(0)$. Therefore, $\vecvalue^\star=\vecvalue^\star=\bar{\ivalue}(0)\bm{1}-e^{-\sink} \bm{W}\circ \bm{\xi}$.
\end{proof}
\begin{remark}
If we assume that $\transition_{\tok\tokk}>0$ for any $\tok$, $\tokk$ and suppose that the initial value $\vecvalue(0)$ is close enough to $\vecvalue^\star$, it is possible to prove the fast convergence of $\vecvalue(t)$ to $\vecvalue^\star$.
\begin{equation*}
\|\vecvalue(t) - \vecvalue^\star\|^2_2 \leq \delta e^{-\mu t}.
\end{equation*}
\end{remark}
