# Supplementary material for: Active-Dormant Attention Heads: Mechanistically Demystifying Extreme-Token Phenomena in LLMs
Source: arXiv:2410.13835 source file (2024-11-07)
Supplement: Supplementary file 9 [file tmp.tex]

\frac{\partial \log\Big[\sum_{\toki=1}^\vocabsize \transition^\tokksup_\toki\exp\Big[\frac{W^\tokisup\beta^\tokisup+e^{\sink_j}\ivalue_\toki}{e^{\sink_j}+W}\Big]\Big]}{\partial \ivalue_\tok} = &~ \frac{e^{\sink_j}}{e^{\sink_j}+W} \cdot \frac{  \transition^\tokksup_\tok \exp\Big[\frac{W^\tokksup\beta^\tokksup+e^{\sink_j}\ivalue_\tok}{e^{\sink_j}+W}\Big]}{\sum_{\toki=1}^\vocabsize \transition^\toksup_\toki\exp\Big[\frac{W^\tokisup\beta^\tokisup+e^{\sink_j}\ivalue_\toki}{e^{\sink_j}+W}\Big]}\label{eqn:ds-part1} \\
\frac{\partial 
